# Supplementary material for: Fast 5DOF Needle Tracking in iOCT
Source: arXiv:1802.06446 source file (2018-02-18)
Supplement: Supplementary file 1 [file appendix.tex]

\section{Relationship between Tool centerline and ellipse parameters}
\color{niceblue}
The relationship between $\cos \alpha$ and $\cos \theta$ follows directly from geometric considerations:

\section{Kalman }
